# Supplementary material for: Non-intrusive and Unconstrained Keystroke Inference in VR Platforms via Infrared Side Channel
Source: arXiv:2412.14815 source file (2024-12-19)
Supplement: Supplementary file 1 [file appendix_testing_sequences.tex]

\begin{table}[ht]
\centering
%\vspace{-15pt}
\scriptsize
\setlength{\tabcolsep}{5pt}

\centering
\begin{tabular}{cccccc}
\toprule
\textbf{Length} & \textbf{Keystrokes}                                   & \textbf{Length} & \textbf{Keystrokes}                                                  & \textbf{Length} & \textbf{Keystrokes}                                                                 \\ \midrule\midrule
1               & \begin{tabular}[c]{@{}c@{}}a\\ c\\ o\end{tabular}             & 6               & \begin{tabular}[c]{@{}c@{}}people\\ should\\ though\end{tabular}             & 11              & \begin{tabular}[c]{@{}c@{}}achievement\\ fancinating\\ celebration\end{tabular}             \\ \midrule
2               & \begin{tabular}[c]{@{}c@{}}it\\ of\\ be\end{tabular}          & 7               & \begin{tabular}[c]{@{}c@{}}however\\ because\\ despite\end{tabular}          & 12              & \begin{tabular}[c]{@{}c@{}}conservation\\ housekeeping\\ neighborhood\end{tabular}          \\ \midrule
3               & \begin{tabular}[c]{@{}c@{}}the\\ and\\ for\end{tabular}       & 8               & \begin{tabular}[c]{@{}c@{}}computer\\ learning\\ document\end{tabular}       & 13              & \begin{tabular}[c]{@{}c@{}}qualification\\ globalization\\ misunderstood\end{tabular}       \\ \midrule
4               & \begin{tabular}[c]{@{}c@{}}that\\ with\\ have\end{tabular}    & 9               & \begin{tabular}[c]{@{}c@{}}beautiful\\ adventure\\ dangerous\end{tabular}    & 14              & \begin{tabular}[c]{@{}c@{}}implementation\\ hypersensitive\\ disappointment\end{tabular}    \\ \midrule
5               & \begin{tabular}[c]{@{}c@{}}would\\ about\\ there\end{tabular} & 10              & \begin{tabular}[c]{@{}c@{}}basketball\\ depression\\ technology\end{tabular} & 15              & \begin{tabular}[c]{@{}c@{}}microelectronic\\ acknowledgement\\ procrastination\end{tabular} \\ \bottomrule
\end{tabular}%
\vspace{0.05in}
\caption{Keystrokes for testing with lengths from $1$ to $15$.}
\label{tab:testing_keystrokes}
\vspace{-0.25in}
\end{table}
